# Supplementary material for: Forecasting Polarized Radio Sources for CMB observations
Source: arXiv:1712.09639 source file (2018-03-01)
Supplement: Supplementary file 1 [file appendix_plots.tex]

\begin{comment}
\begin{figure*}	
	\includegraphics[width=.6\columnwidth]{Lognormal_030GHz}
	\includegraphics[width=.6\columnwidth]{Lognormal_044GHz} 
	\includegraphics[width=.6\columnwidth]{Lognormal_070GHz}\\
	\includegraphics[width=.6\columnwidth]{Lognormal_100GHz}
	\includegraphics[width=.6\columnwidth]{Lognormal_143GHz}
	\includegraphics[width=.6\columnwidth]{Lognormal_217GHz}
   \caption{Lognormal distribution from \pl catalogues PCCS2 .} \label{fig:lognormpl}
\end{figure*}
\begin{figure*}
\includegraphics[width=.6\columnwidth]{Lognormal_NVSS}
\includegraphics[width=.6\columnwidth]{Lognormal_SPASS}
\caption{Lognormal distribution from the Joint SPASS/NVSS catalogue.}\label{fig:lognormspass}
\end{figure*}
\end{comment}
